# Supplementary material for: Approximate Query Service on Autonomous IoT Cameras
Source: arXiv:1909.00841 source file (2020-05-05)
Supplement: Supplementary file 1 [file appendix.tex]

\clearpage

\appendix

\section{CI of single \aggwindow}

According to our Equation~\ref{eq:3} and the observation that operator error distribution is independent from $\mu_x$, we can derive the mean and standard deviation of $\mu$ as following. Here, $\mu_{e1}, \mu_{e2}$ are the mean of the operator error distribution $E_1, E_2$, and $\sigma_{e1}, \sigma_{e2}$ are their standard deviation.

\begin{equation}\label{eq:4}
\begin{split}
\bar{x} > \theta: \\
E(\mu) & = E(\mu_x) \times E(e_1) = \bar{X} \times \mu_{e1}\\
\sigma^2(\mu) & = (E(\mu_x) + \sigma(\mu_x)) \times (E(e_1) + \sigma(e_1)) - E(\mu_x)^2E(e_1)^2 \\
& = (\sigma^2(u_x) + \bar{X}^2)(\mu_{e1}^2+\sigma_{e1}^2) - \bar{X}^2\mu_{e1}^2 \\
\bar{x} \leq \theta:\\
E(\mu) & = E(\mu_x) + E(e_2) = \bar{X} + \mu_{e2}\\
\sigma^2(\mu) & = \sigma^2(u_x) + \sigma_{e2}^2\\
Where:\\
\sigma^2(u_x) & = \frac{S^2}{n} \sigma(t_{n-1}) = \frac{S^2(n-1)^2}{n(n-3)^2}
\end{split}
\end{equation}

%\begin{equation}\label{eq:4}
%E(\mu) =
%   \begin{cases}
%     \bar{X} \times \mu_{e1} & \quad \text{if } \bar{x} > \theta\\
%     \bar{X} + \mu_{e2} & \quad \text{if } \bar{x} \leq \theta
%   \end{cases}\\
%\end{equation}
%\begin{equation}\label{eq:5}
%\sigma^2(\mu) =
%   \begin{cases}
%     (\sigma^2(u_x) + \bar{X}^2)(\mu_{e1}^2+\sigma_{e1}^2) - \bar{X}^2\mu_{e1}^2 & \quad \text{if } \bar{x} > \theta\\
%     \sigma^2(u_x) + \sigma_{e2}^2 & \quad \text{if } \bar{x} \leq \theta
%   \end{cases}\\
%\end{equation}
%\[
%here: \sigma^2(u_x) = \frac{S^2(n-1)^2}{n(n-3)^2}
%\]

Though the distributions of $V_1$ and $V_2$ are non-standard, we observe that they are similar to normal distributions with similar CDF (cumulative distribution function). Thus, we can estiamte the V-value $v_{1, \alpha}, v_{2, \alpha}$ by treating $V_1,V_2$ as a normal distributions with mean $E(\mu)$ and standard deviation $\sigma(\mu)$.

\begin{equation}\label{eq:5}
\begin{split}
& V_1, V_2 \thicksim N(E(\mu), \sigma^2(\mu)) \\
& \Rightarrow \frac{v_1 - E(\mu)}{\sigma(\mu)}, \frac{v_2 - E(\mu)}{\sigma(\mu)} \thicksim N(0, 1) \\
& \Rightarrow v_{1, \alpha}, v_{2, \alpha} = z_{\alpha/2} \sigma(\mu)
\end{split}
\end{equation}

where $z_{\alpha/2}$ is the z-value of normal distribution. Combing Equation~\ref{eq:5} and Equation~\ref{eq:4}, we have the derivation of CI width to the sample number as following.

\begin{equation} \label{eq:7}
\begin{split}
& \frac{\partial v_{1, \alpha}}{\partial n} = z_{\alpha/2}\cdot\frac{2(\mu_{e1}^2+\sigma_{e1}^2)\sigma(\mu_x)}{\sigma(\mu)}\cdot\frac{\partial \sigma(\mu_x)}{\partial n}\\ 
& \frac{\partial v_{2, \alpha}}{\partial n} = z_{\alpha/2}\cdot\frac{2\sigma(\mu_x)}{\sigma(\mu)}\cdot\frac{\partial \sigma(\mu_x)}{\partial n}\\
& here: \frac{\partial \sigma(\mu_x)}{\partial n} = -\frac{n^2+3}{2(n-3)^2n^{\frac{3}{2}}} \cdot S
\end{split}
\end{equation}

\section{CI of multiple {\aggwindow}s}

To build the mean distribution ($\mu_{t}$) of $k$ adjacent {\aggwindow}s ($W_1, W_2, ... W_k$), we can estimate the mean distributions of each individual \aggwindow{} first based on Equation~\ref{eq:6} ($\mu_1, \mu_2, ... \mu_k$). Since each \aggwindow{} has same window size, we can combine them as following.

\begin{equation} \label{eq:8}
\begin{split}
\mu_t & = \frac{1}{k} \sum_{i=1,2,...k} \mu_i \\
& \thicksim N(\frac{1}{k} \sum E(\mu_i), \frac{1}{k^2} \sum \sigma^2(\mu_i))
\end{split}
\end{equation}

The resultant confidence interval is

\[
[\frac{1}{k} \sum E(\mu_i) \quad \pm \quad z_{\alpha / 2} \times \frac{1}{k} \sqrt{\sum \sigma^2(\mu_i)}]
\]

Here, $E(\mu_i)$ and $\sigma(\mu_i)$ are calculated based on Equation~\ref{eq:4} and Equation~\ref{eq:5}. $\alpha$ is the specified confidence level.

\note{Each $\mu_i$ may not be independent. Use covariance.}
